# Supplementary material for: Provably Secure Robust Image Steganography via Cross-Modal Error Correction
Source: arXiv:2412.12206 source file (2024-12-15)
Supplement: Supplementary file 1 [file 6appendix.tex]

\clearpage

\section{Appendix}

\subsection{Visual Quality}

We use ImageNet benchmark under the image resolution of $256\times 256$, which is popular in image reconstruction and generation task.
% 我们使用流行的ImageNet benchmark在256*256分辨率下。
We randomly generate $10,000$ cover and $10,000$ stego images using $1000$ tags in ImageNet. The FID and IS values between them and the original images in the ImageNet dataset are computed separately.
% 我们使用ImageNet中的1k个标签随机生成10000张cover和10000张stego images。分布计算他们与ImageNet数据集中的原始图像间的FID值，计算公式如下：

\begin{table}[h]
\centering
\begin{tabular}{@{}ccc@{}}
\toprule
    & Cover  & Stego \\ \midrule
FID & 19.53 & 19.48 \\
IS  & 415.80 & 414.53 \\ \bottomrule
\end{tabular}
\caption{Quality evaluation of generated images.}\label{tab:fid}
\end{table}

We show more examples of randomly generated cover images using LlamaGen and stego images generated using \name{} embedded random secret messages in Figure~\ref{fig:cover} and Figure~\ref{fig:stego}.

\subsection{Design of Cross-Modal Error-Correction Module}

The effectiveness of the cross-modal error correction module has been verified in Table~\ref{tab:robust}. 
% To further illustrate the effectiveness of the three information compression principles we designed, we additionally tested two error correction information composition methods. One is to use the absolute coordinates of the error location and the correct token value directly without any compression; the second is to compress the coordinates using the relative coordinates and the token value using the ordinal number of the probability value ordering corresponding to the correct token value, again introducing two parameters responsible for controlling the number of information bits.
Below we further illustrate the need for the three information compression principles used in the module.
% 跨模态纠错模块的有效性已经在表2中得到验证。为了进一步说明我们设计的三条信息压缩原则的有效性，我们在额外测试了两种纠错信息构成方式。一是不进行任何压缩，直接使用错误位置的绝对坐标和正确token值；第二种是对坐标使用相对坐标进行压缩，对token值使用正确token值所对应的概率值排序的序号进行压缩，同样引入两个参数负责控制信息位数。

\begin{table}[htbp]
\centering
\begin{tabular}{@{}cccccc@{}}
\toprule
\multicolumn{3}{c}{w/o R.C.} & \multicolumn{3}{c}{w/ R.C.} \\ \midrule
Mean    & Std   & Max   & Mean   & Std   & Max   \\ \midrule
173.61   & 26809.1 & 575  & 11.16   & 35.9 & 496  \\ \bottomrule
\end{tabular}
\caption{Statistics on the amount of information required to transmit a coordinate under different designs.}\label{tab:rc}
\end{table}

\begin{table}[htbp]
\centering
\begin{tabular}{@{}cccccc@{}}
\toprule
\multicolumn{3}{c}{w/o V.P.} & \multicolumn{3}{c}{w/ V.P.} \\ \midrule
Mean    & Std   & Max   & Mean   & Std   & Max   \\ \midrule
146.27  & 86234.6 & 1945  &  62.17  & 117.6 & 1294 \\ \bottomrule
\end{tabular}
\caption{Statistics on the amount of information required to transmit a token value under different designs.}\label{tab:vp}
\end{table}

The first principle, predecessor priority, is easy to understand. Due to the nature of the autoregressive model to predict the next token one by one, any token error that occurs in the front will affect the extraction of message embedded in all the tokens after it. Therefore, prioritizing error correction for the preorder token can maximize the integrity of the message.
% 第二条原则Relative Coordinate，缩写为R.C.，旨在使用相对前一个错误token的位置信息代替绝对坐标，来减少需要传输的位置信息量。
The second principle, Relative Coordinate (R.C.), seeks to minimize the amount of positional information that needs to be transmitted by using coordinates relative to the previous error token rather than absolute positions. As an example, if for a sequence of tokens to be corrected, the error positions are the 24th, 27th, and 35th token. After using the R.C. principle, the positional information to be conveyed is 24, 3, 12 in order. We statistically calculate the coordinate information required for error correction of optimized 50 stego images under JPEG compression noise with a quality factor of 75. As shown in Table~\ref{tab:rc}, the introduction of the R.C. principle can substantially reduce the mean and standard deviation of the amount of information required. 
We perform similar statistics on the effect of the third principle, Vector Proximity (V.P.). Results are shown in Table~\ref{tab:vp}. The top-$k$ value was set to 2000 in the experiment.
The impact of the R.C. and V.P. on the length of the amount of information that needs to be transmitted for coordinate and token value, respectively, is shown in the form of a histogram in Figure~\ref{fig:rcvp}.

% \subsection{Effect of truncation factor on robustness}

% % 从
\begin{figure}[htbp]
    \centering
    \begin{subfigure}{0.48\columnwidth}
        \includegraphics[width=\columnwidth]{figure/appendix/error-rc.png}
        \caption{Coordinate}
    \end{subfigure}
    \begin{subfigure}{0.48\columnwidth}
        \includegraphics[width=\columnwidth]{figure/appendix/error-vp.png}
        \caption{Token indice value}
    \end{subfigure}
    \caption{Comparison of the impact of R.C. and V.P. principles on the length of coordinate and value bits.}
    \label{fig:rcvp}
\end{figure}

We use this as a basis for setting the values of $\lambda_1$ and $\lambda_2$ to $8$, i.e., each value represents $0-255$.

\subsection{Practical Experiments on OSN}

In this section, we validate the practical performance of \name{} on Weibo, a popular Chinese social networking platform, where the uploaded images will suffer from spatial filtering, resize and JPEG recompression. 
The $384\times384$ images will be scaled to $360\times360$ and be compressed.
We randomly select $10$ images and uploaded them onto Weibo. 
We use a noise layer with a quality factor of 80 to simulate channel noise for token optimization and a stego text of length 200 for error correction.
The results are shown in Table~\ref{table:weibo}, demonstrating that our method can be well adapted to the requirements of practical application environments. The results are generalizable due to the existence of all possible lossy processing of OSN in this experiment.

\begin{table}[htbp]
\centering
\begin{tabular}{@{}ccc@{}}
\toprule
\multirow{2}{*}{OSN} & \multicolumn{2}{c}{\name{}} \\ \cmidrule(l){2-3} 
                     & $R_q$       & $Cap$      \\ \midrule
Weibo                & 97.52       & 3340       \\ \bottomrule
\end{tabular}
\caption{Performance of the proposed \name{} on Weibo.}\label{table:weibo}
\end{table}

\begin{figure*}[t]
    \centering
    \includegraphics[width=\textwidth]{figure/appendix/cover.png}
    \caption{Cover images randomly generated by LlamaGen.}
    \label{fig:cover}
\end{figure*}

\begin{figure*}[t]
    \centering
    \includegraphics[width=\textwidth]{figure/appendix/stego.png}
    \caption{Stego images generated by \name{}.}
    \label{fig:stego}
\end{figure*}

\clearpage
